# Supplementary material for: MosaicSets: Embedding Set Systems into Grid Graphs
Source: arXiv:2208.07982 source file (2022-08-16)
Supplement: Supplementary file 1 [file interview.pdf]

# Expert Interview

## Scenario

The board of an institution (e.g., a university faculty) would like to improve its strategic planning processes by supporting discussions in meetings with informative visualizations. In particular, the board would like to visualize the division of its research groups into organizational units (e.g. departments) as well as important intra-institutional collaborations (e.g., major research projects involving several research groups from different departments). It is important that each research group is represented equally. Interactive components can also be used to represent the organizational structures on a web presentation to the public.

## Introduction to our Visualization

In our approach, each research group is represented as a cell on a hexagonal or rectilinear grid. We enforce that all cells of the same department or of a project form a contiguous region. We illustrate the departments by coloring all cells corresponding to one department with the same color. Furthermore, each project is visualized by its region's boundary. We assign a distinct color to each project.

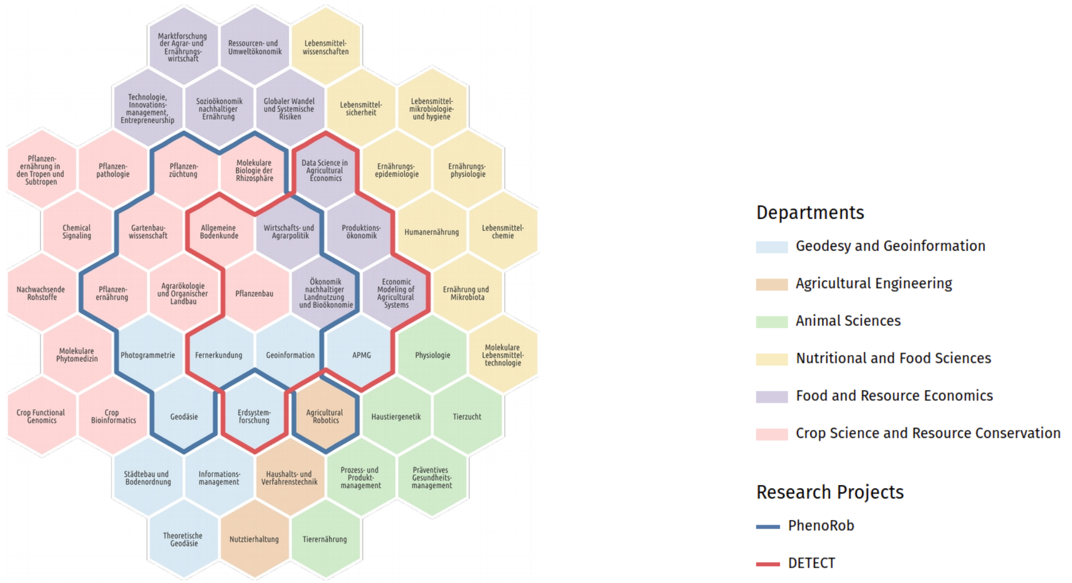


For the web presentation each legend entry is enriched such that a user can select and highlight each department individually. The projects are not displayed by default, but can be added to the visualization manually.

- ➔ Show SVG.

# Rectilinear vs. Hexagonal Grid

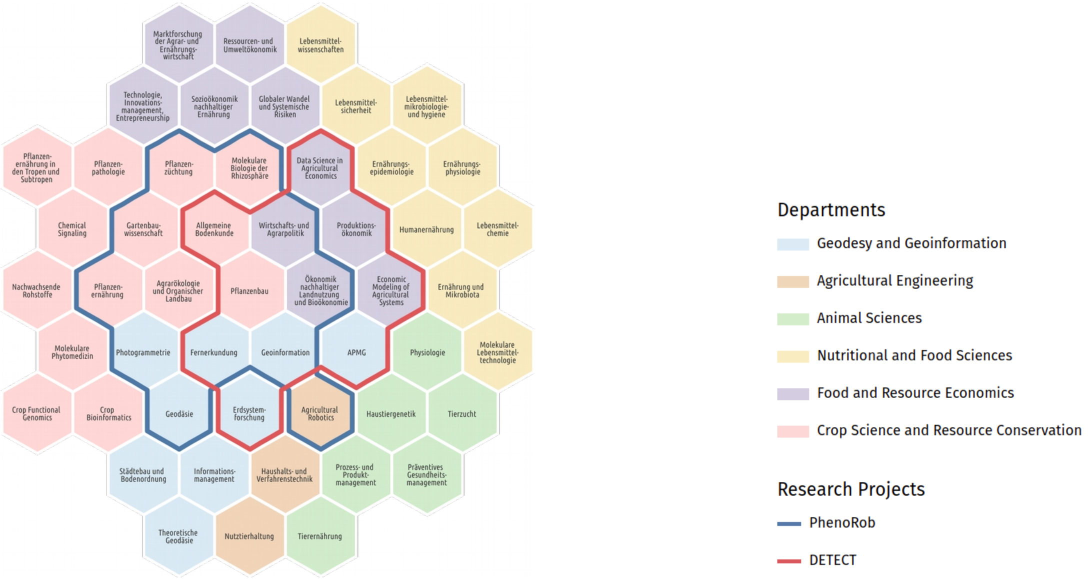


*Figure 1: Hexagonal Grid*

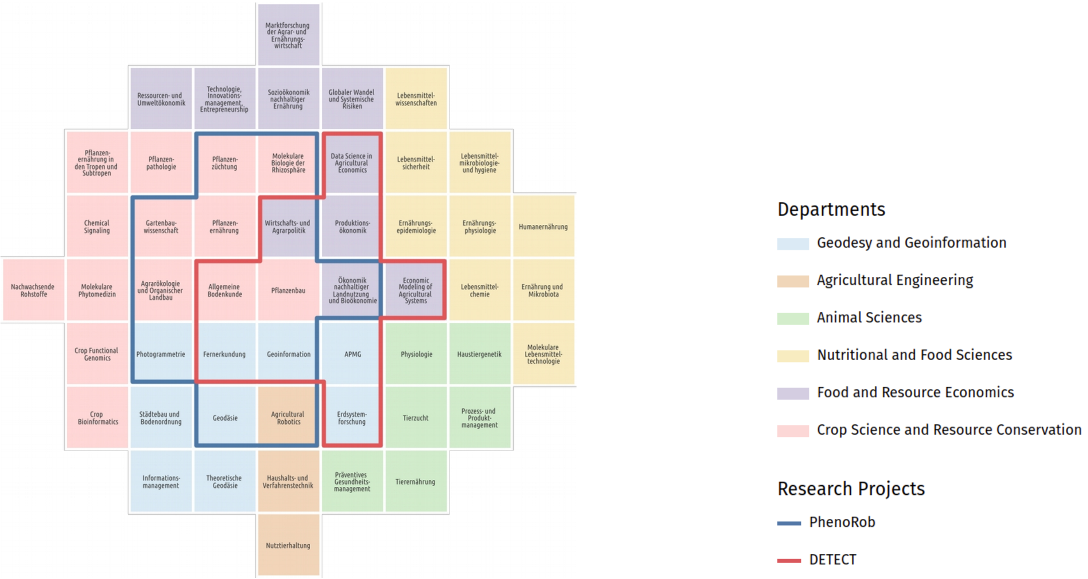


*Figure 2: Rectilinear Grid*

- Which one is visually more appealing?
- Which one is more clear?
- What advantages and disadvantages do you see?

# Comparison of different rendering styles for the projects

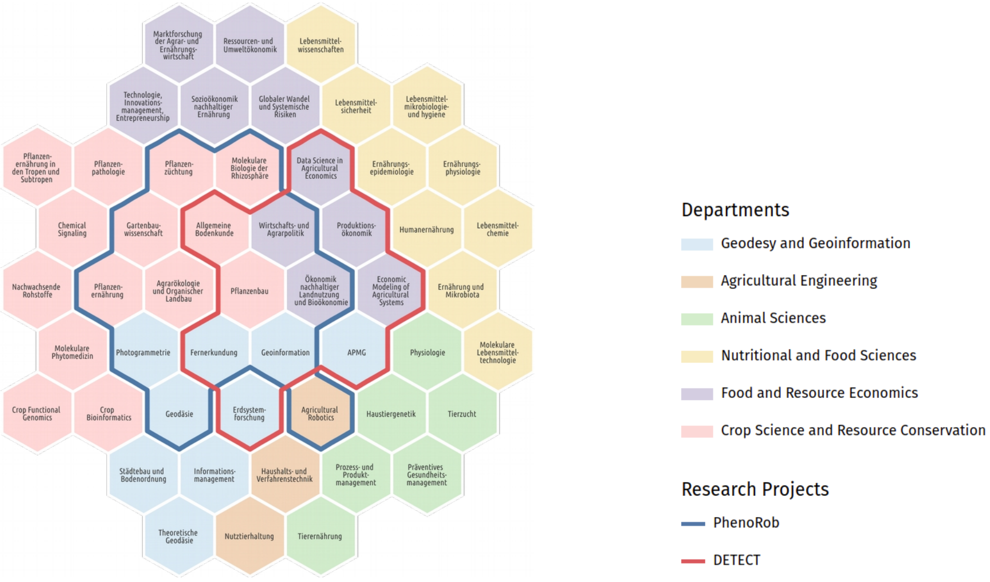


*Figure 3: Projects as Regions*

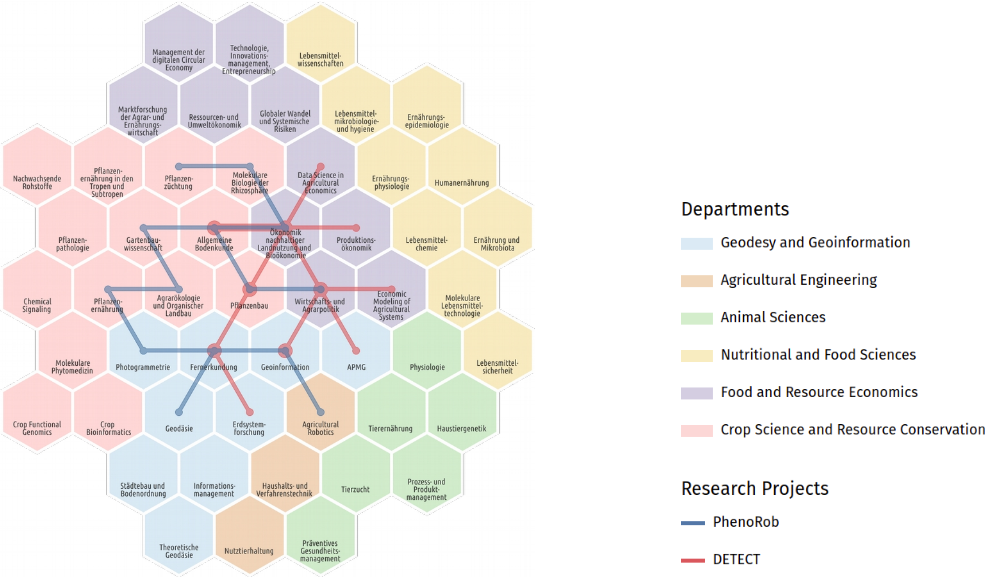


*Figure 4: Kelp-Style*

- Which one is visually more appealing?
- Which one is more clear?
- What advantages and disadvantages do you see?

# Compactness

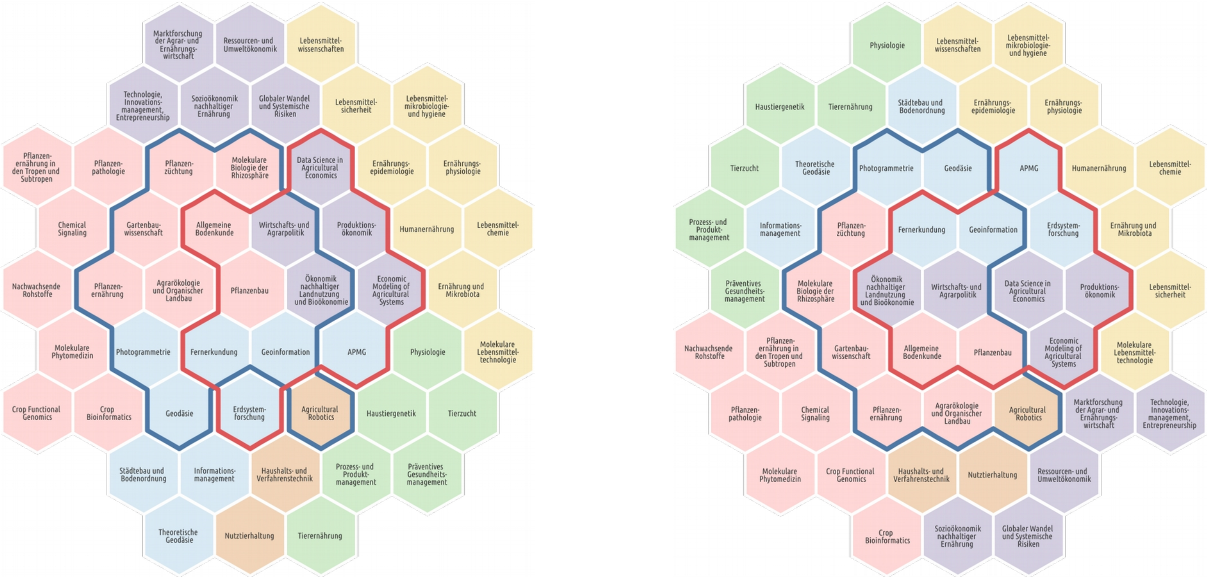


*Figure 5: Left: Compact; Right: Non-Compact.*

- Which one is visually more appealing?
- Which one is more clear?
- What advantages and disadvantages do you see?

# Number of projects for static use-case.

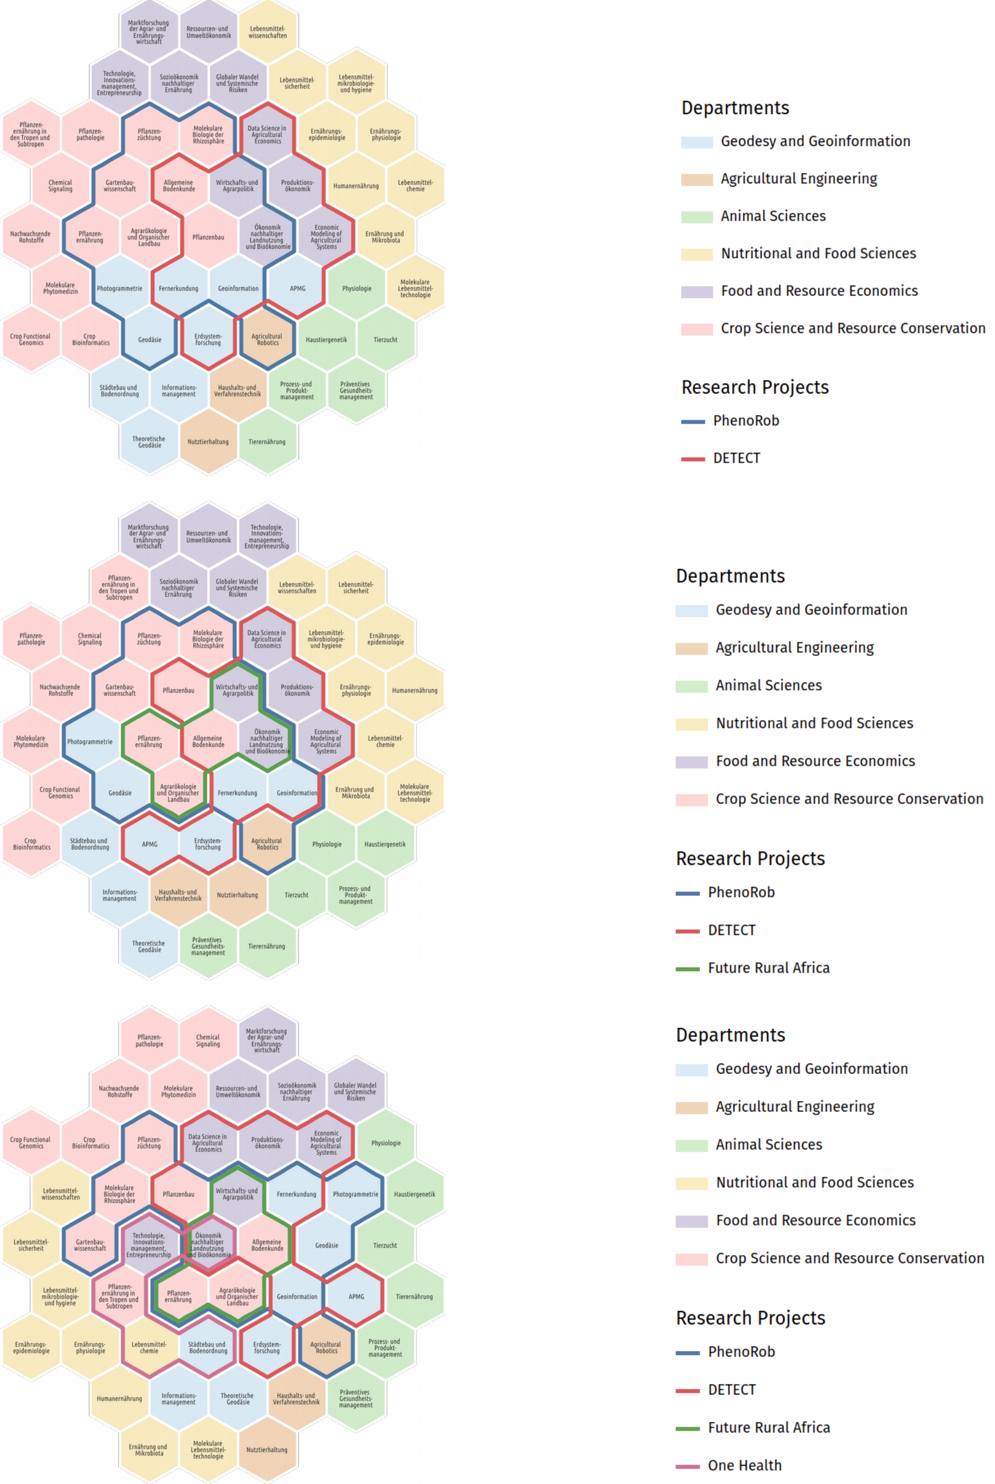


*Figure 6: Visualization with 2, 3 and 4 research projects.*

- The three figures differ in terms of the number of research projects represented. In your opinion, at what number of projects is the limit of what can be clearly presented with our approach?

# Static vs Interactive.

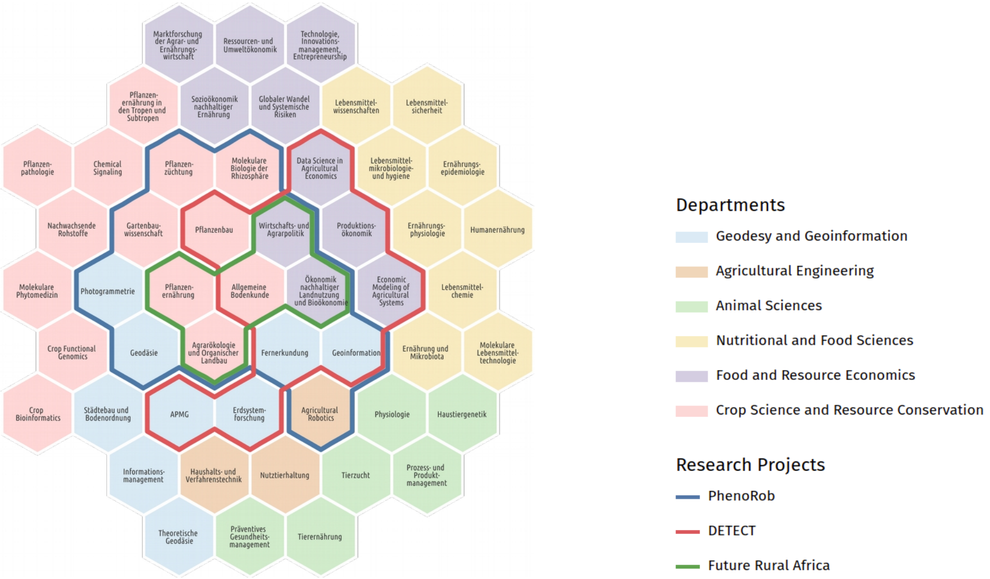


*Figure 7: Static Visualization*

→ show participant the interactive version for comparison

- Can the interactive application improve clarity?
- Do you see any other advantages or disadvantages with the interactive version?

# Comparison to a manually generated visualization by an expert

In the following, we compare a visualization created manually by an expert against a visualization generated by our approach. Please consider only the layout when answering the following questions and do not refer to design elements such as font type and size or color choice.

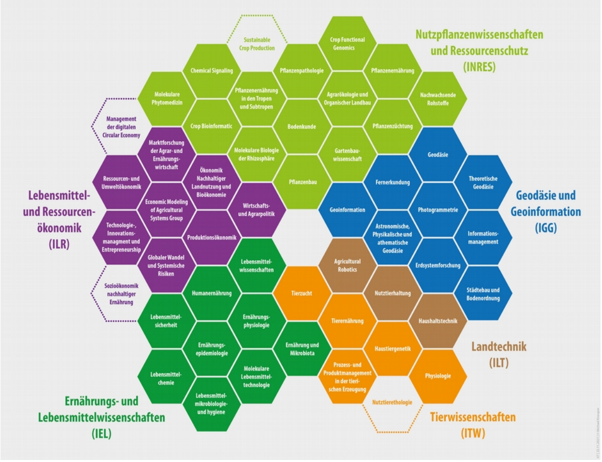


*Figure 8: Manually Generated*

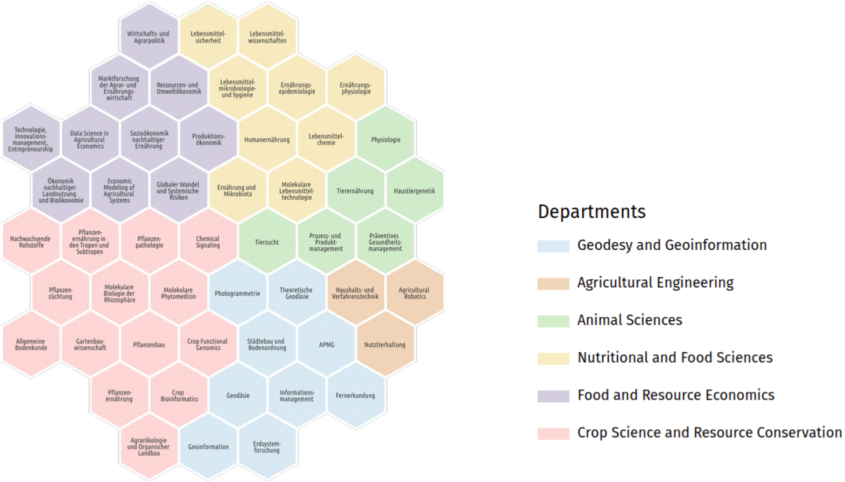


*Figure 9: Our Solution*

- Which layout is visually more appealing?
- Which one is more clear?
- What advantages and disadvantages do you see?

Only to the expert that designed the visualization manually:

- What criteria did you use to create the visualization?
- Are these criteria also sufficiently considered in our visualization?

# Tasks from State-Of-The-Art Paper

When designing a set visualization, it is important to determine which tasks should be supported. To this end, Alsallakh et al. gives a list of general tasks that are supported by existing visualization techniques. In the following, we ask you to classify our visualization with respect to these tasks. For each task you can choose between 'fully supported', 'partially supported' and 'not supported'.

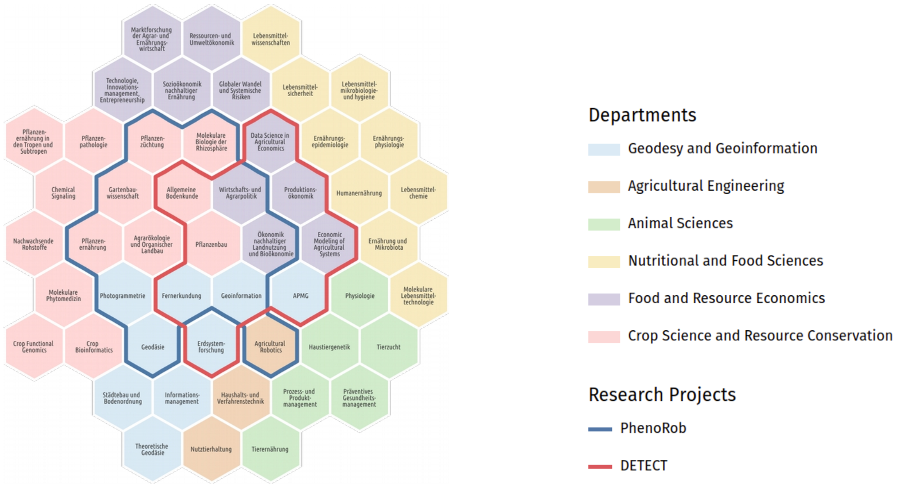


| | *Task* | Fully supported | Partially supported | Not supported |
|---|---|---|---|---|
| *A1* | *Find all research groups that belong to PhenoRob.* | | | |
| *A2* | *Find the department and projects in which the research group 'Photogrammetrie' is contained.* | | | |
| *A3* | *Find all research groups that are part of the IGG but not of PhenoRob.* | | | |
| *A4* | *Find all research groups that are part of one department and two projects.* | | | |
| *A5* | *Show me only research groups in PhenoRob.* | | | x |
| *A6* | *Show me only research groups that are in two projects.* | | | x |
| *A7* | *Create a new set that contains certain elements.* | | | x |
| *B1* | *How many departments and projects exist?* | | | |
| *B2* | *Is PhenoRob included in IGG?* | | | |
| *B3* | *Is PhenoRob included in DETECT, and DETECT in turn is included in IGG?* | | | |
| *B4* | *Do PhenoRob and IEL NOT have a joint research group?* | | | |
| *B5* | *Is there a joint research group of PhenoRob and IGG?* | | | |
| *B6* | *Find the intersection of PhenoRob and IGG.* | | | |

| | | | | |
|---|---|---|---|---|
| | 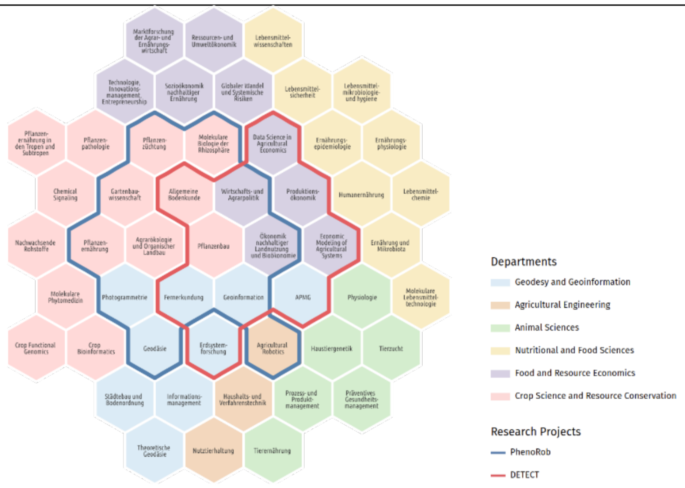 | | | |
| B7 | *Given the following:*<br>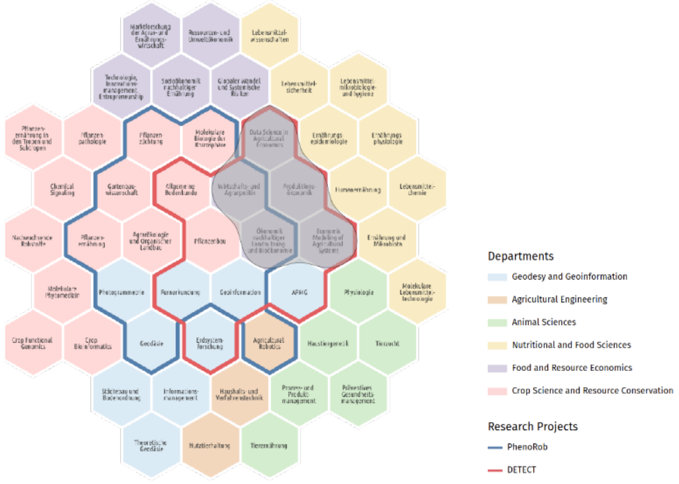<br>*Find the department and projects involved in the intersection (grey).* | | | |
| B8 | *Find all projects in which the IGG is involved.* | | | |
| B9 | *Which department participates in the least/ most projects?* | | | |
| B10 | • *Estimate the number of research groups that are part in PhenoRob and IGG.*<br>• *Compare the number of research groups of ILR and IEL.* | | | |
| B11 | *Analyze and compare set similarities.* | | | x |
| B12 | *Compare the number of IGG research groups not involved in any project to the number of IEL research groups not involved in any project.* | | | |
| B13 | *Highlight sets, subsets or set relations.* | | | x |
| B14 | *Create a new set using set-theoretic operations.* | | | x |

# General Questions

(1) Can you imagine using our visualization for future representations? If this is not the case, what would be necessary?
(2) Where might such visualizations be used within the faculty?
(3) On which occasions (new appointments, new research projects, etc.) would you recreate a visualization? How often do these cases usually occur?
(4) How long may the generation of such a visualization take? For example, is a time of less than one minute sufficient?

Only to the expert that designed the visualization manually:

(1) Approximately how long did it take you to create the visualization?

(2) What limitations do you see?
    a. What additions would you like to see in the visualization?
    b. Regarding the dynamic visualization, what additional interaction options would you like to see?
(3) Is there any further feedback you want to give?
